# Supplementary material for: Privacy Violations in Election Results
Source: arXiv:2308.04100 source file (2025-03-14)
Supplement: Supplementary file 1 [file tab-snyder_ecdf.tex]

\begin{tabular}{rcccccc}
\toprule
 &  & \multicolumn{5}{c}{Voters per 100,000 in units of size:} \\ 
\cmidrule(lr){3-7}
Reporting Unit & Unique units & 1 & $\le 2$ & $\le 5$ & $\le 10$ & $\le 30$\\ 
\midrule\addlinespace[2.5pt]
Precinct & $8,001$ & $0$ & $1$ & $5$ & $12$ & $49$ \\ 
Ballot Style & $4,498$ & $1$ & $2$ & $6$ & $13$ & $46$ \\ 
Precinct $\times$ Ballot Style & $12,465$ & $3$ & $7$ & $16$ & $34$ & $117$ \\ 
Ballot Equivalent & $28,004$ & $10$ & $23$ & $67$ & $158$ & $559$ \\ 
\emph{... only mail method} & $10,173$ & $4$ & $8$ & $20$ & $43$ & $191$ \\ 
\emph{... only in-person method} & $14,787$ & $10$ & $24$ & $71$ & $174$ & $828$\\ 
\emph{... only provisional method} & $3,042$ & $422$ & $983$ & $3,022$ & $7,096$ & $15,991$\\ 
\bottomrule
\end{tabular}
